# Supplementary material for: PathInsight: Instruction Tuning of Multimodal Datasets and Models for Intelligence Assisted Diagnosis in Histopathology
Source: arXiv:2408.07037 source file (2024-08-13)
Supplement: Supplementary file 1 [file appendix_example.tex]

\begin{longtable}

\noindent\rule{\textwidth}{1pt} 
\centering
\textbf{Classification Example}
\noindent\rule{\textwidth}{0.5pt}

\noindent 
\begin{minipage}{0.4\textwidth}
\centering
\includegraphics[width=0.7\linewidth]{fig/result/output_image_8855.jpg}
\end{minipage}
\hfill 
\begin{minipage}{0.5\textwidth}
  Query: Please tell me if cancer cells is present in this image. Answer with yes or no. 
  
  Ground Truth: Yes, this image contains cancerous cells.
\end{minipage}

\noindent 
\begin{minipage}[t]{0.25\textwidth}
    Qwen-VL-Chat
\end{minipage}%
\hfill 
\begin{minipage}[t]{0.75\textwidth}
    yes
\end{minipage}

\noindent
\begin{minipage}[t]{0.25\textwidth}
    Qwen-VL-Insight
\end{minipage}%
\hfill
\begin{minipage}[t]{0.75\textwidth}
    Yes, this image contains cancerous cells. 
\end{minipage}

\noindent 
\begin{minipage}[t]{0.25\textwidth}
    InternLM
\end{minipage}%
\hfill 
\begin{minipage}[t]{0.75\textwidth}
    Yes
\end{minipage}

\noindent 
\begin{minipage}[t]{0.25\textwidth}
    InternLM-Insight
\end{minipage}%
\hfill 
\begin{minipage}[t]{0.75\textwidth}
    Yes, this image contains cancerous cells.
\end{minipage}

\noindent 
\begin{minipage}[t]{0.25\textwidth}
    LLaVA-1.5
\end{minipage}%
\hfill 
\begin{minipage}[t]{0.75\textwidth}
    Yes
\end{minipage}

\noindent\rule{\textwidth}{0.5pt}

\noindent 
\begin{minipage}[t]{0.25\textwidth}
    LLaVA-1.5-Insight
\end{minipage}%
\hfill 
\begin{minipage}[t]{0.75\textwidth}
    Yes, this image contains cancerous cells.
\end{minipage}

\noindent\rule{\textwidth}{0.5pt}

\noindent 
\begin{minipage}{0.4\textwidth}
\centering
\includegraphics[width=0.7\linewidth]{fig/result/DEB-TCGA-LKDRCYAL.png}
\end{minipage}
\hfill 
\begin{minipage}{0.5\textwidth}
  Query: Which category does this pathological images belong to? Choose one of the following categories: 'Adipose', 'Background', 'Debris', 'Lymphocytes', 'Mucus', 'Smooth Muscle', 'Normal Colon Mucosa', 'Cancer-Associated Stroma', 'Colorectal Adenocarcinoma Epithelium'. 
  
  Ground Truth: Debris.
\end{minipage}

\noindent 
\begin{minipage}[t]{0.25\textwidth}
    Qwen-VL-Chat
\end{minipage}%
\hfill 
\begin{minipage}[t]{0.75\textwidth}
    Colorectal Adenocarcinoma Epithelium.
\end{minipage}

\noindent
\begin{minipage}[t]{0.25\textwidth}
    Qwen-VL-Insight
\end{minipage}%
\hfill
\begin{minipage}[t]{0.75\textwidth}
    Debris. 
\end{minipage}

\noindent 
\begin{minipage}[t]{0.25\textwidth}
    InternLM
\end{minipage}%
\hfill 
\begin{minipage}[t]{0.75\textwidth}
    The image appears to be a microscopic view of tissue, possibly cancer-associated stroma.
\end{minipage}

\noindent 
\begin{minipage}[t]{0.25\textwidth}
    InternLM-Insight
\end{minipage}%
\hfill 
\begin{minipage}[t]{0.75\textwidth}
    Debris.
\end{minipage}

\noindent 
\begin{minipage}[t]{0.25\textwidth}
    LLaVA-1.5-Insight
\end{minipage}%
\hfill 
\begin{minipage}[t]{0.75\textwidth}
    Debris.
\end{minipage}

\noindent\rule{\textwidth}{0.5pt}

%-----------------------------------------------------------------------
%3
\noindent 
\begin{minipage}{0.45\textwidth}
  \centering
  \includegraphics[width=0.6\linewidth]{fig/result/MUC-TCGA-HLDWMKMW.png}
\end{minipage}
\hfill 
\begin{minipage}{0.5\textwidth}
  Query: Which category does this pathological images belong to? Choose one of the following categories: 'Adipose', 'Background', 'Debris', 'Lymphocytes', 'Mucus', 'Smooth Muscle', 'Normal Colon Mucosa', 'Cancer-Associated Stroma', 'Colorectal Adenocarcinoma Epithelium' 
  
  Ground Truth: Mucus.
\end{minipage}

\noindent 
\begin{minipage}[t]{0.25\textwidth}
    Qwen-VL-Chat
\end{minipage}%
\hfill 
\begin{minipage}[t]{0.75\textwidth}
    Normal Colon Mucosa.
\end{minipage}

\noindent
\begin{minipage}[t]{0.25\textwidth}
    Qwen-VL-Insight
\end{minipage}%
\hfill
\begin{minipage}[t]{0.75\textwidth}
    Mucus. 
\end{minipage}

\noindent 
\begin{minipage}[t]{0.25\textwidth}
    InternLM
\end{minipage}%
\hfill 
\begin{minipage}[t]{0.75\textwidth}
    The image appears to be a microscopic view of tissue, but without specific details or context, it is difficult to accurately categorize the pathological image.
\end{minipage}

\noindent 
\begin{minipage}[t]{0.25\textwidth}
    InternLM-Insight
\end{minipage}%
\hfill 
\begin{minipage}[t]{0.75\textwidth}
    Normal Colon Mucosa.
\end{minipage}

\noindent 
\begin{minipage}[t]{0.25\textwidth}
    LLaVA-1.5-Insight
\end{minipage}%
\hfill 
\begin{minipage}[t]{0.75\textwidth}
    Mucus.
\end{minipage}

\noindent\rule{\textwidth}{1pt}

\centering
\textbf{Caption Example}
\noindent\rule{\textwidth}{0.1pt}

% \label{tab:your_label}
% \end{table}

%-------------------------------------------------------------------------------------------------

% \begin{table}
% \centering
% \caption{The result of Classification}
% \noindent\rule{\textwidth}{1pt} 
% \centering
% \textbf{Classification Example}
% \noindent\rule{\textwidth}{0.5pt}

%-----------------------------------------------
%5-
\noindent 
\begin{minipage}{0.4\textwidth}
  \centering
  \includegraphics[width=0.75\linewidth]{fig/result/1_00143_sub0_021.png}
\end{minipage}
\hfill 
\begin{minipage}{0.5\textwidth}
  Query: Please describe the primary lesions or abnormalities in this pathology image.
  
  Ground Truth: Moderate pleomorphism and cytologic atypia is present. Nuclei are mildly crowded together. Polarity is completely lost. Mitosis is infrequent throughout the tissue. Prominent nucleoli are easily identified in low magnification scanning. High grade.
\end{minipage}

\noindent 
\begin{minipage}[t]{0.25\textwidth}
    Qwen-VL-Chat
\end{minipage}%
\hfill 
\begin{minipage}[t]{0.75\textwidth}
    The image depicts a micrograph of a human salivary gland tumor. The primary lesion or abnormality in this pathology image is a benign mixed tumor, which is a type of tumor that contains both epithelial and mesenchymal tissue elements...
\end{minipage}

\noindent
\begin{minipage}[t]{0.25\textwidth}
    Qwen-VL-Insight
\end{minipage}%
\hfill
\begin{minipage}[t]{0.75\textwidth}
    Mild pleomorphism and cytologic atypia is present. Mild nuclear crowding is seen. Polarity is completely lost. Mitosis is frequent throughout the tissue. Nucleoli is prominent. High grade. 
\end{minipage}

\noindent 
\begin{minipage}[t]{0.25\textwidth}
    InternLM
\end{minipage}%
\hfill 
\begin{minipage}[t]{0.75\textwidth}
    The primary lesions or abnormalities in this pathology image are the presence of numerous small, round cells with pink cytoplasm and dark nuclei. These cells appear to be densely packed and form a characteristic pattern that is indicative of a specific type of tissue or disease process...
\end{minipage}

\noindent 
\begin{minipage}[t]{0.25\textwidth}
    InternLM-Insight
\end{minipage}%
\hfill 
\begin{minipage}[t]{0.75\textwidth}
    Nuclear features show mild pleomorphism. Mild nuclear crowding is seen. Architecturally the cells show complete lack of polarity toward the surface urothelium. Mitosis is rare. The nucleoli of nuclei are prominent. High grade.
\end{minipage}

\noindent 
\begin{minipage}[t]{0.25\textwidth}
    LLaVA-1.5-Insight
\end{minipage}%
\hfill 
\begin{minipage}[t]{0.75\textwidth}
    Nuclear features show mild pleomorphism. Nuclei are mildly crowded together. Polarity is completely lost. Mitosis is rare throughout the tissue. Nucleoli is prominent. High grade.
\end{minipage}

\noindent\rule{\textwidth}{0.5pt}

\noindent 
\begin{minipage}{0.4\textwidth}
  \centering
  \includegraphics[width=0.55\linewidth]{fig/result/openpath_441.jpg}
\end{minipage}
\hfill 
\begin{minipage}{0.5\textwidth}
  Query: Can you provide a summarize the  lesion in this pathology image patch?
  
  Ground Truth: pleomorphic lobular carcinoma: think histiocytoid or myoid; notable apocrime differentiation (evidenced here with GCDFP-15)
\end{minipage}

\noindent 
\begin{minipage}[t]{0.25\textwidth}
    Qwen-VL-Chat
\end{minipage}%
\hfill 
\begin{minipage}[t]{0.75\textwidth}
    The image shows a patch of brown-stained tissue from a biopsy of a lung tumor. The stain indicates the presence of cancer cells.
\end{minipage}

\vspace{6pt} % 在这里调整距离

\noindent
\begin{minipage}[t]{0.25\textwidth}
    Qwen-VL-Insight
\end{minipage}%
\hfill
\begin{minipage}[t]{0.75\textwidth}
    MYXOINFLAMMATORY FIBROBLASTIC SARCOMALocally aggressive tumor Distal (acral) extremitiesMultinodular growthVariably hyalinized/myxoid stroma Scattered bizarre epithelioid cells with macronucleoliOccasional pseudolipoblasts Mixed inflammatory infiltrate
\end{minipage}

\noindent 
\begin{minipage}[t]{0.25\textwidth}
    InternLM
\end{minipage}%
\hfill 
\begin{minipage}[t]{0.75\textwidth}
    The image displays a microscopic view of tissue, with numerous cells and structures visible. The tissue appears to be densely packed with cells, which are scattered throughout the patch...
    
\end{minipage}

\noindent 
\begin{minipage}[t]{0.25\textwidth}
    InternLM-Insight
\end{minipage}%
\hfill 
\begin{minipage}[t]{0.75\textwidth}
    Pleomorphic liposarcoma.
\end{minipage}

\noindent 
\begin{minipage}[t]{0.25\textwidth}
    LLaVA-1.5-Insight
\end{minipage}%
\hfill 
\begin{minipage}[t]{0.75\textwidth}
    60 yo M w large destructive lytic pelvic bone mass from acetabulum to sacroiliac joint. Hemipelvectomy. Gross pic: https://kikoxp.com/posts/5132. WSI digital slides: https://kikoxp.com/posts/5131. Answer & video: https://kikoxp.com/posts/5306.
\end{minipage}

\noindent\rule{\textwidth}{1pt}

% \label{tab:your_label}
% \end{longtable}
%-----------------------------------------------
%-----------------------------------------------

% \begin{table}
% \centering
% \caption{The result of PathVQA}
% \noindent\rule{\textwidth}{1pt} 
\centering
\textbf{PathVQA Example}
\noindent\rule{\textwidth}{0.5pt}

%5 Caption result
\noindent 
\begin{minipage}{0.4\textwidth}
  \centering
  \includegraphics[width=0.6\linewidth]{fig/result/img_455.jpg}
\end{minipage}
\hfill 
\begin{minipage}{0.5\textwidth}
  Query: What is sloughed off at places with exudate of muco-pus in the lumen ?
  
  Ground Truth: Mucosa.
\end{minipage}

\noindent 
\begin{minipage}[t]{0.25\textwidth}
    Qwen-VL-Chat
\end{minipage}%
\hfill 
\begin{minipage}[t]{0.75\textwidth}
    The lining of the tubule is sloughed off at places with exudate of muco-pus in the lumen.
\end{minipage}

\noindent
\begin{minipage}[t]{0.25\textwidth}
    Qwen-VL-Insight
\end{minipage}%
\hfill
\begin{minipage}[t]{0.75\textwidth}
    the bronchial wall
\end{minipage}

\noindent 
\begin{minipage}[t]{0.25\textwidth}
    InternLM
\end{minipage}%
\hfill 
\begin{minipage}[t]{0.75\textwidth}
    Epithelial cells
\end{minipage}

\noindent 
\begin{minipage}[t]{0.25\textwidth}
    InternLM-Insight
\end{minipage}%
\hfill 
\begin{minipage}[t]{0.75\textwidth}
    Epithelial cells
\end{minipage}

\noindent 
\begin{minipage}[t]{0.25\textwidth}
    LLaVA-1.5-Insight
\end{minipage}%
\hfill 
\begin{minipage}[t]{0.75\textwidth}
    the epithelium
\end{minipage}

\noindent\rule{\textwidth}{0.5pt}

\end{longtable}
