# Supplementary material for: PathInsight: Instruction Tuning of Multimodal Datasets and Models for Intelligence Assisted Diagnosis in Histopathology
Source: arXiv:2408.07037 source file (2024-08-13)
Supplement: Supplementary file 2 [file appendix_prompt.tex]

\textbf{Prompts for image captioning.} The prompts used for image captioning are detailed in Table 1. These prompts are specifically designed to draw out detailed descriptions of pathological images, emphasizing the identification of key features and abnormalities.

\begin{table}[h]\centering\includegraphics[width=\textwidth]{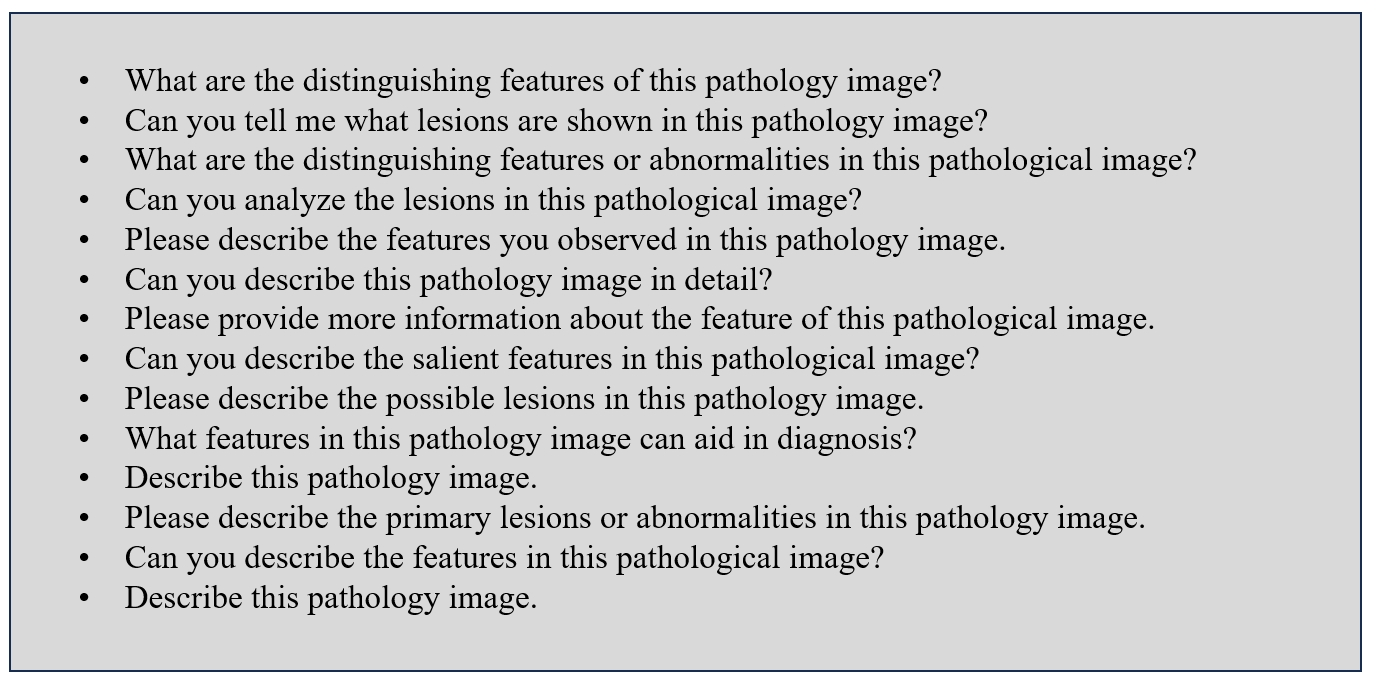}\caption{List of prompts for image captioning.}\label{table5}\end{table}

\textbf{Prompts for classification.} The prompts used for classification tasks are presented in Table 2. These prompts focus on assigning the image to specific predefined categories and detecting the presence of cancerous cells.

\begin{table}[h]\centering\includegraphics[width=\textwidth]{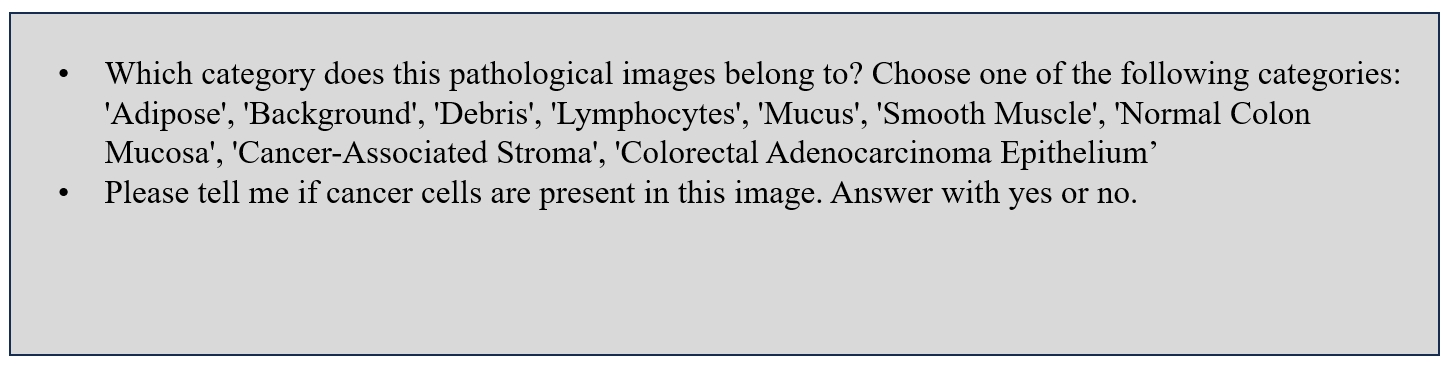}\caption{List of prompts for classification.}\label{table6}\end{table}
